# Supplementary material for: Zero-shot Depth Completion via Test-time Alignment with Affine-invariant Depth Prior
Source: arXiv:2502.06338 source file (2025-02-10)
Supplement: Supplementary file 1 [file scenenet.tex]

\begin{figure*}[t]
\centering
   \includegraphics[width=0.85\linewidth]{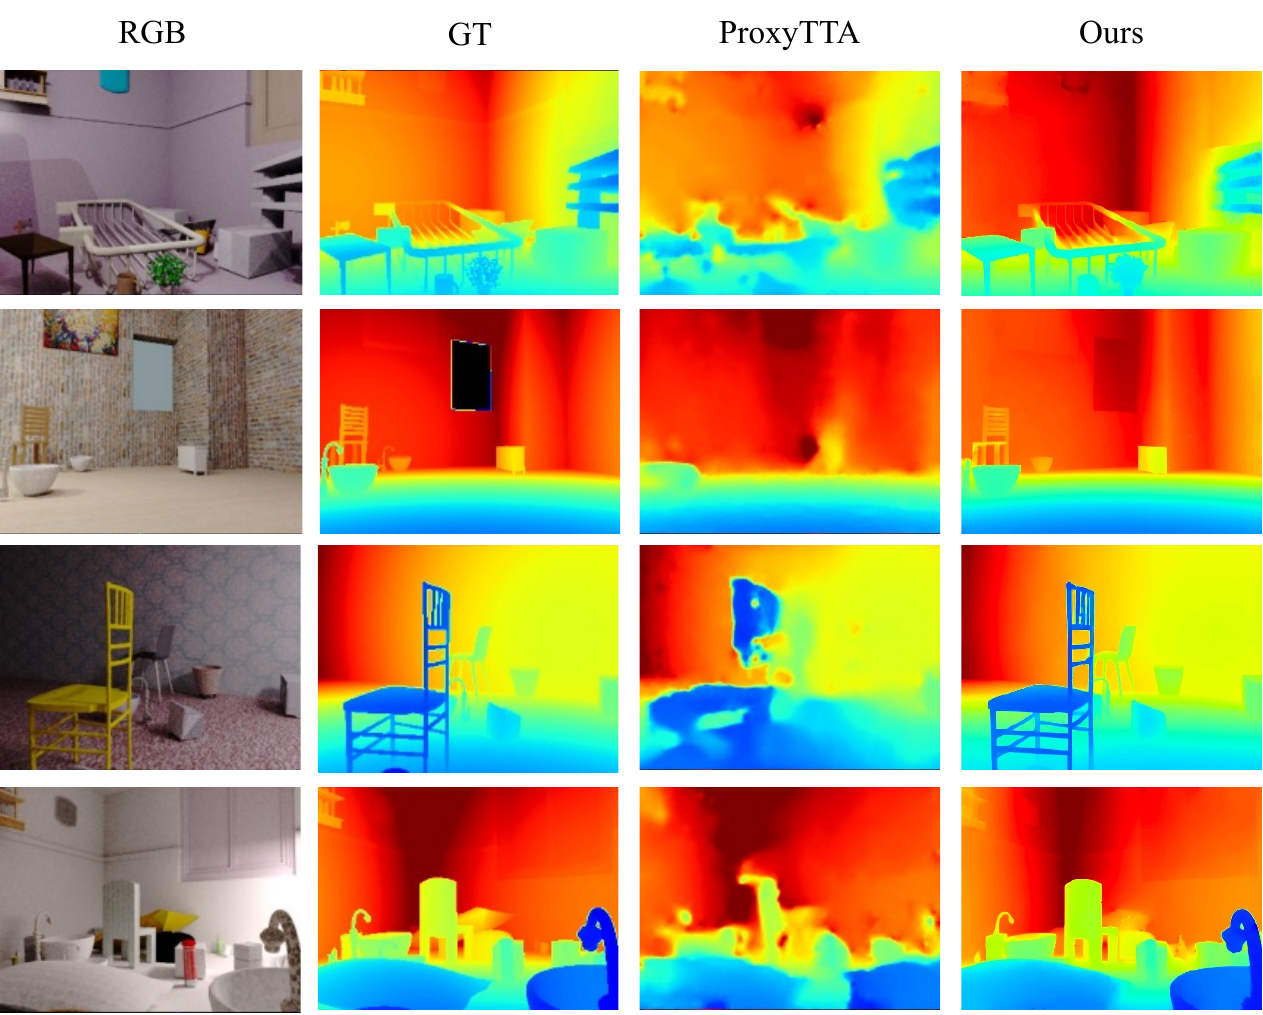}
   \caption{\textbf{Qualitative results on SceneNet}} 
\label{fig:qual_scenenet}
\end{figure*}
